# Supplementary material for: Implicit Geometry of Next-token Prediction: From Language Sparsity Patterns to Model Representations
Source: arXiv:2408.15417 source file (2025-02-19)
Supplement: Supplementary file 1 [file additional_exps.tex]

\pagebreak
\section{Additional Experiments for camera ready}
\tina{@Yize: get rid of this section when figures moved}
\subsection{Experiments}
\subsubsection{Sim(H,H) with context labels(appendix)}
To demonstrate the connection between geometries of context embeddings and semantic meanings, we include the labeled pairwise similarity matrix for smaller-scale datasets. (Figure \ref{fig:sim_H_lable_404}, \ref{fig:sim_H_label_verysmall})
For example, in our synthetic setting(Figure \ref{fig:sim_H_label_verysmall}), we show higher similarities between the embedding of "Lily was playing with her" and "lily spent time with her". \yz{should I include S heatmap with labels as well}

\subsubsection{MLP (main body experimental section)}
To verify the geometry properties in other architectures, we trained a Multi-layer Perceptron model(MLP) on Extracted TinyStories dataset. As MLP models are less expressive than Transformers, we use a MLP contained eight times more number of parameters comparing to transformers. 
\yz{say something about the result}
% \begin{figure}
%     \centering
%     \includegraphics[width=1\linewidth]{exp_results_yize/Sim_SHWFixedLMLP_d128.pdf}
%     \caption{\yz{fix:remove title, fix colorbar. }Embedding geometries trained by MLP. \\First row: Geometry Comparison between $S$ and $\Hb$; second row: Geometry comparison between $S^T$ and $W^T$ }
%     \label{fig:Sim_SHWFixedLMLP_d128}
% \end{figure}
\subsubsection{Auto-regressive Loss curve(Auto-regressive section in the appendix)+explain in the set-up}
Note that the length of context does not have impact on our theory, therefore we expect similar behavior in Auto-regressive(AR) setting, where we vary the context length. 
For this experiment, we train a 8-layer transformer auto-regressively on 200 stories from TinyStories with character-level tokenizer. We measure the loss convergence to entropy 
at each position from t=2 to t=17, i.e. for context length from 1 to 16. 
We also compare the pairwise-similarity of different length context embeddings and their pairwise similarity of support sets.

\subsubsection{Additional Linear Layer Experiment}
This section examines the network's performance when the decoder dimension $d_{\text{decode}}$ is less than $V$, contrary to the requirement of $d>V$ specified in Equation \ref{eq:ufm relax}. By fixing the context embeddings' expressibility, we investigate the impact of varying $d_{\text{decode}}$ on the geometry embeddings. To maintain adequate expressivity, we configure the network with ten transformer layers, each with a dimensionality of $d=64$. Additionally, we introduce an extra linear layer to adjust $d_{\text{decode}}$, and subsequently, we analyze the effects on loss convergence and geometric properties.

\begin{figure}[ht]
\centering
\vspace{-10pt}
\begin{subfigure}{0.6\textwidth}
		\centering
  \hspace{-55pt}
		\begin{tikzpicture}
			\node at (-0,-0) 
			{\includegraphics[scale=0.3]{exp_results_yize/Hsim_6 layer Transformer pos off_d64.pdf}};
   \node at (0.0,-1.7) [scale=0.9]{(a) cosine similarity heatmaps};
		\end{tikzpicture}
    \end{subfigure}
    \hspace{35pt}
    \begin{subfigure}{0.3\textwidth}
		\centering
		\begin{tikzpicture}
			\node at (-0,-0) 
			{\includegraphics[scale=0.33]{exp_results_yize/CEloss_6layerTFM_tiny_extract_m404_128_64.pdf}};
   \node at (0.0,-1.7) [scale=0.9]{(b) loss convergence};
		\end{tikzpicture}
    \end{subfigure}
    \caption{\textbf{(a)} Left: Column-wise similarities of support sets.  Middle and Right: Column-wise similarities of context embeddings $H$ trained with Transformer model with $d=128>V$ and $d=64<V$, respectively. The vocabulary size is set to $V=104$, and number of unique contexts $m=403$, \textbf{(b)} Loss converges to lower bound $H=1.2179$ for both transformer models with $d=128>V$ and $d=64<V$.}

    \label{fig:d<V}
    \end{figure}
\subsubsection{SSIM curves \yz{(Include!!) for W as well, in the main body}}
% \subsubsection{SSIM Curves}
We quantitatively measure the structural similarity index (SSIM), as defined in \eqref{eq:ssim}, between the cosine similarities of $Cos(H, H)$, $Cos(S, S)$, $Cos(W^T, W^T)$, and $Cos(S^T, S^T)$ throughout the training process. This analysis complements the patterns observed in the heatmaps regarding the embedding geometry.

% \begin{figure}[h]
%     \centering
%     \begin{tikzpicture}
%         % Node for the first image
%         \node[anchor=south west,inner sep=0] (image1) at (0,0) {\includegraphics[width=0.5\textwidth]{exp_results_yize/H_S_sim_structural_corr_bothdatasets.pdf}};
%         % Node for the second image, right next to the first
%         \node[anchor=south west,inner sep=0] (image2) at (image1.south east) {\includegraphics[width=0.5\textwidth]{exp_results_yize/W_S_sim_structural_corr_bothdatasets.pdf}};
%     \end{tikzpicture}
%     \caption{Increasing structural correlation between $Cos(H, H)$ and $Cos(S, S)$, as well as $Cos(W^T, W^T)$ and $Cos(S^T, S^T)$, during training. \tina{@Yize: fix title/labels + For the experiments we include in the main body, I prefer to have their ssim in the main body. or is Appendix better?} \tina{$SS^\top$ or the centered one?}}
% \end{figure}

% \begin{figure}
%     \centering
%     \includegraphics[width=1\linewidth]{exp_results_yize/H_S_sim_structural_corr_bothdatasets.pdf}
%     \caption{Increasing structural correlation between $Cos(H, H)$ and $Cos(S, S)$ during training.}
%     \label{fig:H_S_sim_ssim}
% \end{figure}
% \begin{figure}
%     \centering
%     \includegraphics[width=1\linewidth]{exp_results_yize/W_S_sim_structural_corr_bothdatasets.pdf}
%     \caption{Increasing structural correlation between $Cos(W^T, W^T)$, and $Cos(S^T, S^T)$ during training.}
%     \label{fig:W_S_sim_ssim}
% \end{figure}

\subsubsection{SSIM for conjecture \yz{?}}

 \pagebreak
